# Supplementary material for: Understanding temperature-dependent SU($3$) spin dynamics in the $S=1$ antiferromagnet Ba$_2$FeSi$_2$O$_7$
Source: arXiv:2205.11770 source file (2022-05-24)
Supplement: Supplementary file 1 [file Supplementary_information.pdf]

# Supplementary Information for “Understanding temperature-dependent SU(3) spin dynamics in the $S = 1$ antiferromagnet $\text{Ba}_2\text{FeSi}_2\text{O}_7$ ”

Seung-Hwan Do<sup>1,\*</sup>, Hao Zhang<sup>1,2,\*</sup>, David A. Dahlbom<sup>2</sup>, Travis J. Williams<sup>3</sup>, V. Ovidiu Garlea<sup>3</sup>, Tao Hong<sup>3</sup>, Tae-Hwan Jang<sup>4</sup>, Sang-Wook Cheong<sup>4,5</sup>, Jae-Hoon Park<sup>4,6</sup>, Kipton Barros<sup>7</sup>, Cristian D. Batista<sup>2,†</sup>, and Andrew D. Christianson<sup>1,‡</sup>

<sup>1</sup>Materials Science and Technology Division, Oak Ridge National Laboratory, Oak Ridge, Tennessee 37831, USA

<sup>2</sup>Department of Physics and Astronomy, University of Tennessee, Knoxville, Tennessee 37996, USA

<sup>3</sup>Neutron Scattering Division, Oak Ridge National Laboratory, Oak Ridge, Tennessee 37831, USA

<sup>4</sup>MPPHC-CPM, Max Planck POSTECH/Korea Research Initiative, Pohang 37673, Republic of Korea

<sup>5</sup>Rutgers Center for Emergent Materials and Department of Physics and Astronomy, Rutgers University, Piscataway, New Jersey 08854, USA

<sup>6</sup>Department of Physics, Pohang University of Science and Technology, 37673, Republic of Korea

<sup>7</sup>Theoretical Division and CNLS, Los Alamos National Laboratory, Los Alamos, New Mexico 87545, USA

\*These authors contributed equally to this work

†cbatist2@utk.edu

‡christiansad@ornl.gov

## ABSTRACT

### 1 Background subtraction

Figure S1(a-e) show the original INS spectrum with temperatures for  $[H, 0, 0.5]$  direction. Noticeably, there appears to be strong quasi-elastic scattering below 0.5 meV in low  $Q$ -region is attributed. This quasi-elastic scattering is temperature independent, and arises from the incompletely blocked direct beam due to the oscillating collimator of the HYSPEC spectrometer. To subtract the background, the quasi-elastic scattering was modeled with a single Gaussian function centered at  $\sim E = 0$  meV and the function was fitted to the 90 K spectrum. The extracted background spectrum is shown in Fig. S1(f). This background was subtracted from the other temperature data, and the resulting spectrum are shown in Fig.2(a) of the main text. The background subtracted spectra for  $[H, 0, 0.5]$  exhibit almost identical spectra collected at different ZC,  $\mathbf{Q} = (1, 0, 1.5)$ , which confirms that the background subtraction works correctly.

### 2 Monte Carlo simulation on $\text{CP}^2$

To obtain the dynamical spin structure factor at finite temperatures, we must generate an ensemble of initial states of the spin-one system by sampling from the Boltzmann distribution  $P \propto e^{-E/(k_B T)}$  with  $E = \langle Z | \mathcal{H} | Z \rangle$  for the GLLD. This is achieved by applying the standard Metropolis-Hastings Monte Carlo (MC) algorithm. The classical limit discussed in this paper is based on direct products of SU(3) coherent states

$$|Z\rangle = \otimes_{\mathbf{r}} |Z_{\mathbf{r}}\rangle, \quad (1)$$

where the coherent state on a particular site  $\mathbf{r}$  is parameterized with four angles

$$|Z_{\mathbf{r}}\rangle = \cos \theta_{\mathbf{r}} |0\rangle + e^{i\alpha_{1,\mathbf{r}}} \sin \theta_{\mathbf{r}} \cos \phi_{\mathbf{r}} |1\rangle + e^{i\alpha_{2,\mathbf{r}}} \sin \theta_{\mathbf{r}} \sin \phi_{\mathbf{r}} |-1\rangle, \quad (2)$$

The resulting manifold of coherent states is  $S^5/S^1 \sim \text{CP}^2$ . The “local MC move” must be uniformly distributed on  $S^5/S^1$ , which is achieved by applying the inverse transform sampling method, i.e. generating a local random move from the cumulative distribution function of the angle parameters:

$$\theta = \sin^{-1}(U_1^{1/4}), \phi = \sin^{-1}(U_2^{1/2}), \alpha_{1,2} = 2\pi U_{3,4}, \quad (3)$$

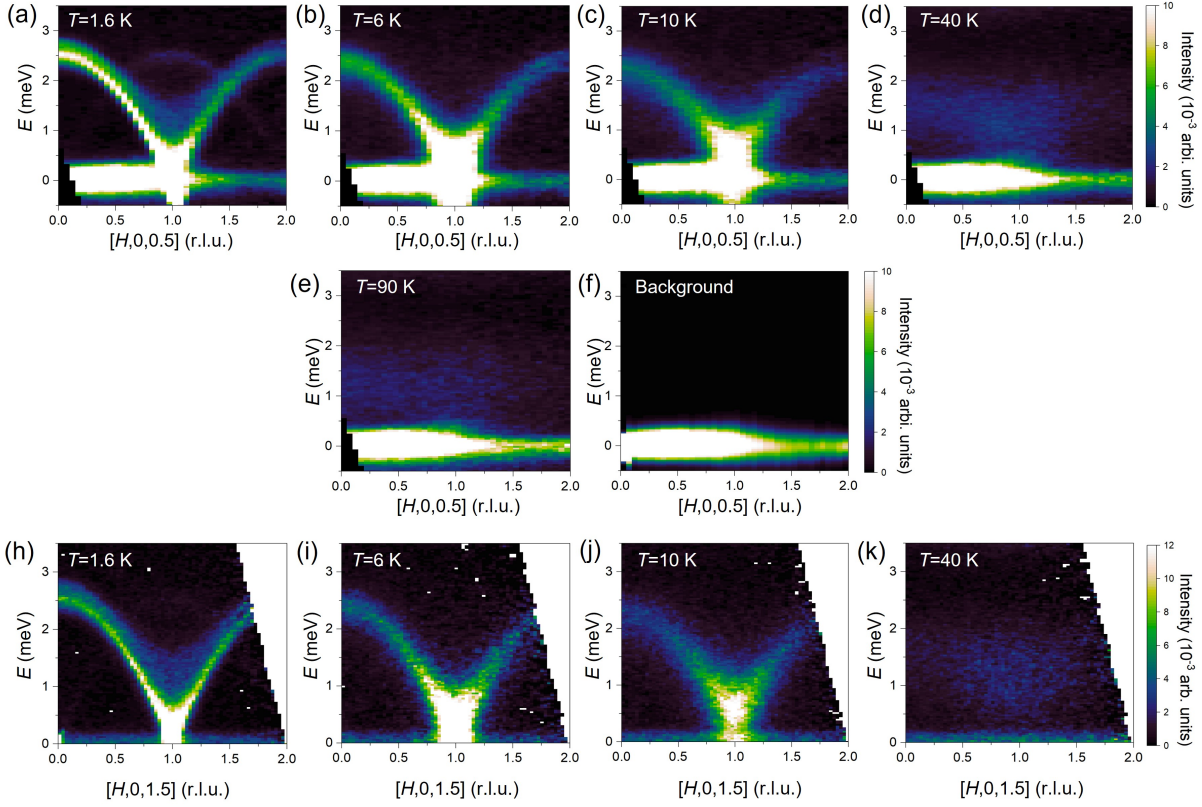

**Figure S1.** (a-e) Original INS spectra measured at  $T = 1.6$  K, 6 K, 10 K, 40 K, and 90 K for  $[H, 0, 0.5]$  direction. (f) Extracted quasi-elastic background scattering by fitting the Gaussian function to 90 K spectrum. (h-k) Original INS spectra at same temperatures for  $[H, 0, 1.5]$  direction.

where  $U_{1,2,3,4}$  are pseudo-random numbers uniformly distributed between zero and one. Once the system is thermalized, we save the angle snapshots every 100 MC sweeps (the interval of 100 sweeps is greater than the autocorrelation time of  $\simeq 60$  MC sweeps). These snapshots are used to compute expectation values of the eight SU(3) generators:

$$\begin{aligned}
 o_{\mathbf{r}}^1 &= \frac{\sqrt{2}}{2} \sin 2\theta_{\mathbf{r}} [\cos \alpha_{1,\mathbf{r}} \cos \phi_{\mathbf{r}} + \cos \alpha_{2,\mathbf{r}} \sin \phi_{\mathbf{r}}] \\
 o_{\mathbf{r}}^2 &= \frac{\sqrt{2}}{2} \sin 2\theta_{\mathbf{r}} [-\sin \alpha_{1,\mathbf{r}} \cos \phi_{\mathbf{r}} + \sin \alpha_{2,\mathbf{r}} \sin \phi_{\mathbf{r}}] \\
 o_{\mathbf{r}}^3 &= \sin^2 \theta_{\mathbf{r}} \cos 2\phi_{\mathbf{r}} \\
 o_{\mathbf{r}}^4 &= \frac{\sqrt{2}}{2} \sin 2\theta_{\mathbf{r}} [-\cos \alpha_{1,\mathbf{r}} \cos \phi_{\mathbf{r}} + \cos \alpha_{2,\mathbf{r}} \sin \phi_{\mathbf{r}}] \\
 o_{\mathbf{r}}^5 &= \frac{\sqrt{2}}{2} \sin 2\theta_{\mathbf{r}} [\sin \alpha_{1,\mathbf{r}} \cos \phi_{\mathbf{r}} + \sin \alpha_{2,\mathbf{r}} \sin \phi_{\mathbf{r}}] \\
 o_{\mathbf{r}}^6 &= \cos(\alpha_{1,\mathbf{r}} - \alpha_{2,\mathbf{r}}) \sin^2 \theta_{\mathbf{r}} \sin 2\phi_{\mathbf{r}} \\
 o_{\mathbf{r}}^7 &= -\sin(\alpha_{1,\mathbf{r}} - \alpha_{2,\mathbf{r}}) \sin^2 \theta_{\mathbf{r}} \sin 2\phi_{\mathbf{r}} \\
 o_{\mathbf{r}}^8 &= -\frac{1 + 3 \cos 2\theta_{\mathbf{r}}}{2\sqrt{3}}.
 \end{aligned} \tag{4}$$

These expectation values are used as initial conditions for the GSD.

### 3 Numerical integration of the classical equation of motion

For the results shown in Fig. (2) and (3) of the main text ( $\kappa = 1$ ), we used the fourth-order Runge-Kutta (RK4) method with  $\delta t = 0.01 \text{ meV}^{-1}$  (the step size of the integration, which is small enough to guarantee that the energy is a constant up to the

six digits during the simulation) and  $\tau = 100 \text{ meV}^{-1}$  (time interval of the evolution, which is longer than any characteristic time of the system). For simulations with renormalized SU(3) spins ( $\kappa = 2$ , see Fig. (4) of the main text), we mapped the classical EOM (see Eq. 2 of the main text) to a mean-field Schrödinger dynamics and used the implicit midpoint method (with  $\delta t = 0.12 \text{ meV}^{-1}$  and  $\tau = 580 \text{ meV}^{-1}$ ), which is symplectic and therefore avoids energy drift<sup>1</sup>. We note that it is more difficult to reach the same level of accuracy with the RK4 method for the renormalized SU(3) spins due to the corresponding renormalization in the model parameters.

## 4 Dynamical spin structure factor

In the classical limit, the dynamical spin structure factor is computed as<sup>2</sup>

$$S^{\mu\nu}(\mathbf{Q}, \omega) = \frac{\tau}{2\pi} \sum_{\text{IC}} s^{\mu}(\mathbf{Q}, \omega) s^{\nu}(-\mathbf{Q}, -\omega), \quad (5)$$

where the sum runs over the ensemble of initial conditions obtained from the MC procedure discussed in Sec. 2 and

$$s^{\mu}(\mathbf{Q}, \omega) = \frac{1}{\sqrt{N_s}} \sum_{\mathbf{r}} \frac{1}{\tau} \sum_t e^{-i\mathbf{Q} \cdot \mathbf{r} + i\omega t} s^{\mu}(\mathbf{r}, t) \quad (6)$$

is the Fourier transform of the classical dipolar operator  $s^{\mu}(\mathbf{r}, t)$ , which is obtained from the GSD [ $s^{x,y,z}(\mathbf{r}, t) = o^{1,2,3}(\mathbf{r}, t)$ ] and  $N_s$  is the total number of spins.

Finally, we have verified that the sum rule  $\int d\omega S^{\mu\nu}(\mathbf{Q}, \omega) = S^{\mu\nu}(\mathbf{Q})$ , which relates the integration of the dynamical spin structure factor and the static spin structure factor obtained from MC, is satisfied to a good approximation for the number of initial conditions that we are using. For the results shown in this work, we used 200 and 2000 initial conditions for temperatures below and above  $T_N$ , respectively.

## References

1. Dahlbom, D. *et al.* Geometric integration of classical spin dynamics via a mean-field Schrödinger equation, DOI: [10.48550/ARXIV.2204.07563](https://doi.org/10.48550/ARXIV.2204.07563) (2022).
2. Zhang, H. & Batista, C. D. Classical spin dynamics based on SU( $N$ ) coherent states. *Phys. Rev. B* **104**, 104409, DOI: [10.1103/PhysRevB.104.104409](https://doi.org/10.1103/PhysRevB.104.104409) (2021).
